# Supplementary material for: Dark Energy Survey Year 3 results: cosmology with moments of weak lensing mass maps -- validation on simulations
Source: arXiv:1911.05568 source file (2019-11-13)
Supplement: Supplementary file 1 [file Appendix_old.tex]

\section{Impact of higher order effect on convergence moments}\label{highorder}

We verify here that a number of higher-order corrections to our theoretical modeling has a negligible impact on our cosmological constrains \citep{Schneider1998,Schneider2002b,Krause2009,Schmidt2009}.
We look at three different effects: reduced shear,source-lens clustering and lens bias. 
The former is due to the fact that we cannot directly observe the shear field; in practice, the observed shear has an additional contribution that can be modeled as:

\begin{equation}
\label{A1}
\gamma_{obs} \rightarrow \gamma_{obs}(1+\kappa).
\end{equation}

Moreover, when we observe along a given line of sight we are affected by fluctuations in the density field:

\begin{equation}
\label{A2}
\gamma_{obs} \rightarrow \gamma_{obs}(1+\delta_{obs}).
\end{equation}.

The fluctuations in the density field are due source galaxies overdensities and lensing magnification effects, and at first order can be written as:
\begin{equation}
\delta_{obs} =\delta_{gal} + q\kappa,
\end{equation}
where $q = 2\beta_{f} +\beta_r -2$, and $\beta_{f}$ and$ \beta_r$ are the logarithmic sploes of the flux and size distributions,

\begin{equation}
\beta_f = - \left.\frac{\partial ln n_{obs}}{\partial ln f}\right\rvert_{f=f_{min},r=r_{min}},
\end{equation}
\begin{equation}
\beta_r = - \left.\frac{\partial ln n_{obs}}{\partial ln r}\right\rvert_{f=f_{min},r=r_{min}}.
\end{equation}
Summing up eqs. \ref{A1} \ref{A2}:
\begin{equation}
\label{eq:highorder}
\gamma_{obs} = \gamma[1+\delta_g+(1+q)\kappa].
\end{equation}

Reduced shear contributes as $\approx 1+\kappa$, magnification effects as  $\approx 1+q\kappa$  (with q of the order of $\mathcal{O}(unity)$), lens-source clustering as $\approx 1+\delta_g$. To test the impact of these effects, we used \cite{Takahashi2017} simulations. First, for every redshift layer of the simulations, we generated shear field distribution using the fully-sky spherical harmonics approach laid out in $\S$ \ref{sect:Map Making}. Secondly, we generated shear field distributions for every layer adding (sepratedly) a $1+\kappa$ and $1+delta_g$ contributions. We finally stacked layers together according to the redshift distributions of the WL tomographic bins. This provides us three different shear maps with 1) no high order effect, 2) reduced shear contributions 3) source-lens clustering contributions.
To better study source-lens clustering effects, instead of directly applying the correction to the shear maps, we also generated a galaxy catalog starting from the lens layer of the simulation. We assumed the same number density as in DES, and no bias $b=1$ for the sample. We assigned a shear (with no high order effects) to every galaxy depending on their redshift and their position, and then we made the shear maps for every tomographic bin. We note that when making the map, as we average the shear along the line of sight of a given pixel, we partially cancel source-clustering effects:

\begin{equation}
\avg{\gamma}_{pix(\theta)} \approx \frac{\int dz n(z)(1+\delta(z,\theta)) \gamma(z,\theta)}{\int dz n(z)(1+\delta(z,\theta))}.
\end{equation}

The impact of such corrections on E modes are  shown in fig. \ref{fig:high_order}. We estimated the moments from a  full-sky, noise-free realization of the simulation. We do not show error bars for the moment measurement as they are much smaller then DES Y3 error bars (see fig. ). We do not show magnification effects as they are of the same order of reduced-shear correction. In all cases, such corrections are much smaller then DES Y3 uncertainties. We not that source-lens clustering contribution is reduced when the map making process is included.

\begin{figure}
\begin{center}
\includegraphics[width=0.45 \textwidth]{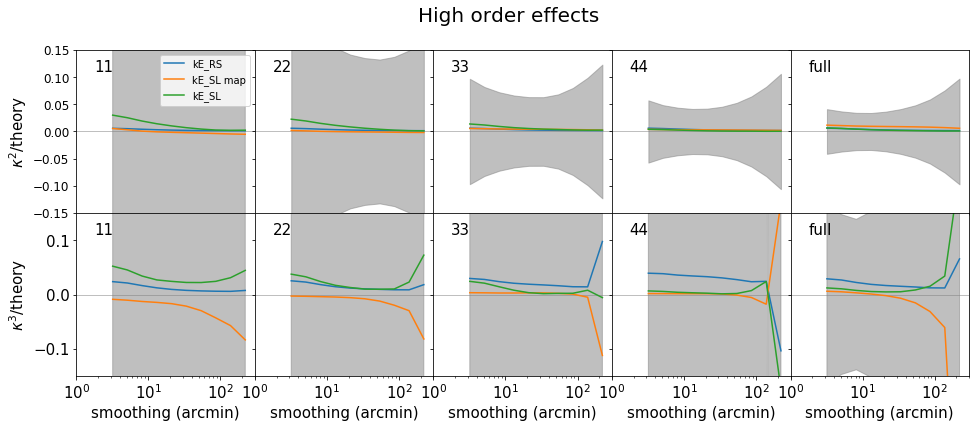}
\end{center}
\caption{Impact of higher order corrections to measured (E-modes) moments. The blue line refers to reduced shear correction. The green line refers to source-lens clustering contribution when applied directly to the shear field, while the orange line includes the map making process (see text for more details). The shaded region shows DES Y3 error bars. }
\label{fig:high_order}
\end{figure}
